# Supplementary material for: Fast generation of Schr\"odinger cat states in a Kerr-tunable superconducting resonator
Source: arXiv:2308.14676 source file (2023-08-28)
Supplement: Supplementary file 1 [file refer_supp.tex]

@book{b28,
author = {Haroche, Serge and Raimond, J.},
year = {2006},
title = {Exploring the Quantum: Atoms, Cavities, and Photons},
publisher = {Oxford Univ Pr}
}
@article{b32,
author = {Wang, Chen and Gao, Yvonne and Reinhold, Philip and others},
year = {2016},
month = {01},
pages = {},
title = {A Schrodinger Cat Living in Two Boxes},
volume = {352},
journal = {Science},
doi = {10.1126/science.aaf2941}
}
@article{b40,
author = {Xue, Hang and Lin, Zhirong and Wenbing, Jiang and others},
year = {2021},
month = {03},
pages = {},
title = {Fabrication and characterization of all-Nb lumped-element Josephson parametric amplifiers},
volume = {30},
journal = {Chinese Physics B},
doi = {10.1088/1674-1056/abeee6}
}
@article{b18,
	doi = {10.1038/s41586-020-2587-z},
  
	url = {https://doi.org/10.1038%2Fs41586-020-2587-z},
  
	year = 2020,
	month = {aug},
  
	publisher = {Springer Science and Business Media {LLC}
},
  
	volume = {584},
  
	number = {7820},
  
	pages = {205--209},
  
	author = {A. Grimm and N. E. Frattini and S. Puri and others},
  
	title = {Stabilization and operation of a Kerr-cat qubit},
  
	journal = {Nature}
}
